# Supplementary material for: Precision spectroscopy of high rotational states in H_2 investigated by Doppler-free two-photon laser spectroscopy in the EF^1\Sigma_g^+ - X^1\Sigma_g^+ system
Source: arXiv:1301.0403 source file (2013-01-03)
Supplement: Supplementary file 1 [file SupMat_Table_I.pdf]

# Precision spectroscopy of high rotational states in $H_2$ investigated by Doppler-free two-photon laser spectroscopy in the $EF^1\Sigma_g^+ - X^1\Sigma_g^+$ system

G. D. Dickenson[1], E. J. Salumbides[1,2], M-L. Niu[1]
Ch. Jungen[3], S. C. Ross[4,5], and W. Ubachs[1]
[1] Department of Physics and Astronomy, LaserLaB, VU University, de Boelelaan 1081, 1081HV, Amsterdam, The Netherlands
[2] Department of Physics, University of San Carlos, Cebu City 6000, The Philippines
[3] Laboratoire Aimé Cotton du CNRS, Bâtiment 505 Université de Paris-Sud, F-91405 Orsay, France
[4] Department of Physics and Centre for Laser, Atomic, and Molecular Sciences, University of New Brunswick, P. O. Box 4400 Fredericton NB, Canada E3B 5A3
[5] Infrared Free Electron Laser Research Center, Tokyo University of Science, 2641 Yamazaki, Noda, Chiba 278-8510, Japan

July 24, 2012

## 1 Supplementary Material: Table 1

Table 1: ($J$=0) Calculated and observed $H_2$ *singlet gerade* $e-$symmetry level energies (in $cm^{-1}$) between 90000 and 112000 $cm^{-1}$.[a]

| state | $J$ | calculated MQDT | observed Bailly *et al.*[b] | obs-calc | observed present | obs-calc | channel character[d] s | d | p |
|---|---|---|---|---|---|---|---|---|---|
| *EF* | 0 | 99161.14[c] | 99164.79 | 3.65 | 99164.79 | 3.65 | 0.930 | 0.014 | 0.056 |
| | 0 | 99365.22 | 99363.89 | -1.33 | | | 0.023 | 0.033 | 0.944 |
| | 0 | 100563.13 | 100558.85 | -4.28 | | | 0.026 | 0.041 | 0.933 |
| | 0 | 101489.78 | 101494.74 | 4.96 | 101494.70 | 4.92 | 0.915 | 0.030 | 0.054 |
| | 0 | 101703.92 | 101698.95 | -4.97 | | | 0.032 | 0.059 | 0.909 |
| | 0 | 102781.01 | 102778.23 | -2.78 | | | 0.043 | 0.105 | 0.852 |
| | 0 | 103558.60 | 103559.60 | 1.00 | 103559.58 | 0.98 | 0.675 | 0.137 | 0.188 |
| | 0 | 103839.17 | 103838.57 | -0.60 | | | 0.144 | 0.130 | 0.726 |
| | 0 | 104734.87 | 104730.59 | -4.28 | | | 0.133 | 0.237 | 0.630 |
| | 0 | 105384.48 | 105384.91 | 0.43 | 105384.90 | 0.42 | 0.427 | 0.090 | 0.483 |
| | 0 | 105962.85 | 105966.15 | 3.30 | | | 0.269 | 0.117 | 0.614 |
| | 0 | 106710.95 | 106713.05 | 2.10 | | | 0.219 | 0.085 | 0.696 |
| | 0 | 107421.68 | 107425.84 | 4.16 | | | 0.271 | 0.098 | 0.631 |
| | 0 | 108092.87 | 108098.48 | 5.62 | | | 0.264 | 0.074 | 0.663 |
| | 0 | 108788.24 | 108793.51 | 5.27 | | | 0.208 | 0.121 | 0.671 |
| | 0 | 109487.65 | 109493.86 | 6.21 | | | 0.216 | 0.069 | 0.714 |
| | 0 | 110156.25 | 110163.34 | 7.10 | | | 0.231 | 0.109 | 0.660 |
| | 0 | 110787.97 | 110794.16 | 6.18 | | | 0.238 | 0.067 | 0.695 |
| | 0 | 111375.16 | 111370.66 | -4.50 | | | 0.205 | 0.184 | 0.611 |
| *GK* | 0 | 111635.42 | 111628.81 | -6.61 | | | 0.423 | 0.209 | 0.368 |
| | 0 | 111811.65 | 111812.63 | 0.98 | | | 0.176 | 0.718 | 0.106 |

[a] The Table compares *ab initio* theoretical level energies with far more accurate experimental energies. The energies have therefore been rounded to two digits after the decimal point throughout, even in cases where the experimental energies have been determined more accurately (cf. Table II of the published paper). [b] D. Bailly, E. Salumbides, M. Vervloet, and W. Ubachs, Mol. Phys. **108**, 827 (2009). [c] The vibronic energies are given in ascending order for each $J$ value. [d] The channel denomination refers to the orbital angular momentum of the outer electron. The full labels are, respectively, $1\sigma_g\epsilon s\sigma$, $1\sigma_g\epsilon d\lambda$ ($\lambda = 0-2$), and $1\sigma_u\epsilon p\lambda$ ($\lambda = 0-1$). [e] Probable misassignment. [f] Tentative assignment.

Table 1: ($J$=1) Calculated and observed $H_2$ *singlet gerade* $e-$symmetry level energies (in $cm^{-1}$) between 90000 and 112000 $cm^{-1}$.

| state | $J$ | calculated MQDT | observed Bailly *et al.*[b] | obs-calc | observed present | obs-calc | channel character[c] s | d | p |
|---|---|---|---|---|---|---|---|---|---|
| $EF$ | 1 | 99224.58 | 99228.22 | 3.64 | 99228.22 | 3.64 | 0.924 | 0.021 | 0.055 |
| | 1 | 99377.46 | 99376.05 | -1.41 | | | 0.023 | 0.033 | 0.944 |
| | 1 | 100575.13 | 100570.84 | -4.29 | | | 0.026 | 0.041 | 0.933 |
| | 1 | 101549.08 | 101554.03 | 4.94 | 101553.95 | 4.87 | 0.918 | 0.024 | 0.058 |
| | 1 | 101715.79 | 101710.85 | -4.94 | | | 0.032 | 0.060 | 0.908 |
| | 1 | 102792.88 | 102790.14 | -2.74 | | | 0.043 | 0.104 | 0.853 |
| | 1 | 103605.15 | 103605.61 | 0.46 | 103605.61 | 0.46 | 0.618 | 0.174 | 0.207 |
| | 1 | 103857.95 | 103857.85 | -0.11 | 103857.92 | -0.03 | 0.172 | 0.126 | 0.702 |
| | 1 | 104751.52 | 104747.34 | -4.17 | | | 0.128 | 0.240 | 0.632 |
| | 1 | 105415.05 | 105415.26 | 0.21 | 105415.28 | 0.23 | 0.412 | 0.101 | 0.488 |
| | 1 | 105987.78 | 105991.22 | 3.44 | | | 0.278 | 0.117 | 0.605 |
| | 1 | 106732.06 | 106734.23 | 2.17 | | | 0.215 | 0.099 | 0.686 |
| | 1 | 107445.49 | 107449.62 | 4.13 | | | 0.267 | 0.100 | 0.632 |
| | 1 | 108116.51 | 108122.17 | 5.66 | | | 0.266 | 0.073 | 0.661 |
| | 1 | 108809.20 | 108814.78 | 5.58 | | | 0.190 | 0.198 | 0.611 |
| | 1 | 109508.45 | 109514.65 | 6.19 | | | 0.214 | 0.070 | 0.716 |
| | 1 | 110177.96 | 110185.07 | 7.11 | | | 0.225 | 0.124 | 0.651 |
| | 1 | 110808.88 | 110815.18 | 6.30 | | | 0.241 | 0.066 | 0.692 |
| | 1 | 111391.64 | 111387.14 | -4.50 | | | 0.183 | 0.289 | 0.529 |
| $GK$ | 1 | 111657.07 | 111650.29 | -6.78 | | | 0.398 | 0.236 | 0.366 |
| | 1 | 111807.63 | 111805.11 | -2.52 | | | 0.170 | 0.721 | 0.109 |

Table 1: ($J$=2) Calculated and observed $H_2$ *singlet gerade* $e-$symmetry level energies (in $cm^{-1}$) between 90000 and 112000 $cm^{-1}$.

| state | $J$ | calculated MQDT | observed Bailly *et al.*[b] | obs-calc | observed present | obs-calc | channel character[c] s | d | p |
|---|---|---|---|---|---|---|---|---|---|
| $EF$ | 2 | 99350.93 | 99354.56 | 3.62 | 99354.56 | 3.63 | 0.928 | 0.017 | 0.054 |
| | 2 | 99401.92 | 99400.51 | -1.40 | | | 0.023 | 0.033 | 0.945 |
| | 2 | 100599.11 | 100594.81 | -4.30 | | | 0.025 | 0.041 | 0.933 |
| | 2 | 101666.85 | 101671.64 | 4.79 | 101671.49 | 4.64 | 0.892 | 0.029 | 0.078 |
| | 2 | 101739.80 | 101735.03 | -4.77 | | | 0.039 | 0.083 | 0.879 |
| | 2 | 102816.56 | 102813.88 | -2.68 | | | 0.042 | 0.102 | 0.856 |
| | 2 | 103691.06 | 103690.15 | -0.91 | 103690.18 | -0.88 | 0.359 | 0.441 | 0.200 |
| | 2 | 103901.81 | 103902.98 | 1.18 | 103903.07 | 1.26 | 0.264 | 0.113 | 0.623 |
| | 2 | 104784.16 | 104780.22 | -3.94 | | | 0.120 | 0.243 | 0.637 |
| | 2 | 105474.19 | 105473.97 | -0.22 | | | 0.326 | 0.246 | 0.427 |
| | 2 | 106038.86 | 106042.55 | 3.69 | | | 0.295 | 0.118 | 0.587 |
| | 2 | 106774.13 | 106776.45 | 2.32 | | | 0.214 | 0.096 | 0.690 |
| | 2 | 107492.48 | 107496.53 | 4.05 | | | 0.259 | 0.108 | 0.634 |
| | 2 | 108163.84 | 108169.58 | 5.74 | | | 0.270 | 0.071 | 0.659 |
| | 2 | 108851.82 | 108857.38 | 5.56 | | | 0.205 | 0.147 | 0.648 |
| | 2 | 109549.73 | 109555.90 | 6.17 | | | 0.211 | 0.070 | 0.718 |
| | 2 | 110221.05 | 110228.17 | 7.12 | | | 0.203 | 0.199 | 0.598 |
| | 2 | 110850.98 | 110857.51 | 6.54 | | | 0.247 | 0.065 | 0.688 |
| | 2 | 111425.15 | 111420.67 | -4.48 | | | 0.215 | 0.201 | 0.585 |
| $GK$ | 2 | 111701.20 | 111693.73 | -7.48 | | | 0.364 | 0.266 | 0.371 |
| | 2 | 111832.99 | 111827.73 | -5.26 | | | 0.167 | 0.712 | 0.121 |

Table 1: ($J$=3) Calculated and observed $H_2$ *singlet gerade* $e-$symmetry level energies (in $cm^{-1}$) between 90000 and 112000 $cm^{-1}$.

| state | $J$ | calculated MQDT | observed Bailly *et al.*[b] | obs-calc | observed present | obs-calc | channel character[c] s | d | p |
|---|---|---|---|---|---|---|---|---|---|
| *EF* | 3 | 99438.57 | 99437.17 | -1.40 | | | 0.023 | 0.032 | 0.945 |
| | 3 | 99539.16 | 99542.77 | 3.60 | 99542.77 | 3.61 | 0.929 | 0.015 | 0.055 |
| | 3 | 100635.04 | 100630.71 | -4.33 | | | 0.025 | 0.041 | 0.934 |
| | 3 | 101773.47 | 101768.58 | -4.89 | | | 0.039 | 0.060 | 0.901 |
| | 3 | 101844.47 | 101849.40 | 4.93 | 101849.34 | 4.87 | 0.823 | 0.023 | 0.154 |
| | 3 | 102851.62 | 102849.36 | -2.59 | | | 0.041 | 0.099 | 0.860 |
| | 3 | 103793.07 | 103789.98 | -3.10 | 103790.09 | -2.98 | 0.291 | 0.274 | 0.434 |
| | 3 | 103992.07 | 103995.21 | 3.15 | 103995.28 | 3.21 | 0.491 | 0.079 | 0.431 |
| | 3 | 104831.94 | 104828.40 | -3.54 | | | 0.112 | 0.242 | 0.646 |
| | 3 | 105557.62 | 105556.84 | -0.78 | 105556.77 | -0.85 | 0.339 | 0.136 | 0.525 |
| | 3 | 106118.43 | 106122.36 | 3.93 | | | 0.320 | 0.119 | 0.561 |
| | 3 | 106837.08 | 106839.67 | 2.59 | | | 0.213 | 0.102 | 0.685 |
| | 3 | 107561.37 | 107565.33 | 3.96 | | | 0.244 | 0.126 | 0.631 |
| | 3 | 108234.83 | 108240.63 | 5.80 | | | 0.272 | 0.076 | 0.652 |
| | 3 | 108915.81 | 108921.54 | 5.73 | | | 0.126 | 0.488 | 0.386 |
| | 3 | 109610.93 | 109617.07 | 6.14 | | | 0.207 | 0.073 | 0.720 |
| | 3 | 110284.76 | 110291.84 | 7.08 | | | 0.193 | 0.219 | 0.588 |
| | 3 | 110914.71 | 110921.60 | 6.89 | | | 0.253 | 0.065 | 0.682 |
| | 3 | 111476.89 | 111472.53 | -4.35 | | | 0.248 | 0.140 | 0.612 |
| *GK* | 3 | 111768.65 | 111759.94 | -8.71 | | | 0.346 | 0.255 | 0.399 |
| | 3 | 111899.95 | 111893.08 | -6.87 | | | 0.138 | 0.744 | 0.118 |

Table 1: ($J$=4) Calculated and observed $H_2$ *singlet gerade* $e-$symmetry level energies (in $cm^{-1}$) between 90000 and 112000 $cm^{-1}$.

| state | $J$ | calculated MQDT | observed Bailly *et al.*[b] | obs-calc | observed present | obs-calc | channel character[c] s | d | p |
|---|---|---|---|---|---|---|---|---|---|
| *EF* | 4 | 99487.37 | 99485.97 | -1.40 | | | 0.023 | 0.032 | 0.945 |
| | 4 | 99787.75 | 99791.33 | 3.58 | 99791.32 | 3.57 | 0.925 | 0.015 | 0.060 |
| | 4 | 100682.87 | 100678.51 | -4.36 | | | 0.025 | 0.040 | 0.935 |
| | 4 | 101821.02 | 101816.13 | -4.89 | | | 0.031 | 0.061 | 0.908 |
| | 4 | 102076.08 | 102081.03 | 4.95 | 102080.91 | 4.83 | 0.919 | 0.027 | 0.054 |
| | 4 | 102898.93 | 102896.46 | -2.47 | | | 0.040 | 0.095 | 0.865 |
| | 4 | 103880.49 | 103876.38 | -4.12 | | | 0.149 | 0.221 | 0.630 |
| | 4 | 104156.07 | 104159.81 | 3.74 | 104159.81 | 3.74 | 0.698 | 0.050 | 0.253 |
| | 4 | 104894.74 | 104891.69 | -3.05 | | | 0.107 | 0.243 | 0.651 |
| | 4 | 105659.03 | 105657.71 | -1.33 | | | 0.287 | 0.149 | 0.564 |
| | 4 | 106228.94 | 106232.93 | 3.99 | | | 0.345 | 0.123 | 0.532 |
| | 4 | 106921.52 | 106924.53 | 3.01 | | | 0.215 | 0.116 | 0.669 |
| | 4 | 107650.40 | 107654.28 | 3.88 | | | 0.201 | 0.239 | 0.559 |
| | 4 | 108328.94 | 108334.75 | 5.81 | | | 0.269 | 0.089 | 0.642 |
| | 4 | 109001.73 | 109007.73 | 6.00 | | | 0.218 | 0.140 | 0.641 |
| | 4 | 109691.50 | 109697.64 | 6.14 | | | 0.203 | 0.079 | 0.719 |
| | 4 | 110367.77 | 110374.76 | 7.00 | | | 0.211 | 0.110 | 0.679 |
| | 4 | 111000.29 | 111007.61 | 7.32 | | | 0.255 | 0.068 | 0.677 |
| | 4 | 111549.00 | 111544.97 | -4.03 | | | 0.271 | 0.146 | 0.582 |
| *GK* | 4 | 111855.32 | 111845.25 | -10.07 | | | 0.320 | 0.254 | 0.426 |

Table 1: ($J$=5) Calculated and observed $H_2$ *singlet gerade* $e-$symmetry level energies (in $cm^{-1}$) between 90000 and 112000 $cm^{-1}$.

| state | $J$ | calculated MQDT | observed Bailly *et al.*[b] | obs-calc | observed present | obs-calc | channel character[c] s | d | p |
|---|---|---|---|---|---|---|---|---|---|
| *EF* | 5 | 99548.26 | 99546.87 | | | | 0.022 | 0.032 | 0.946 |
| | 5 | 100094.71 | 100098.26 | 3.56 | 100098.26 | 3.55 | 0.908 | 0.016 | 0.076 |
| | 5 | 100742.53 | 100738.13 | -4.40 | | | 0.025 | 0.040 | 0.935 |
| | 5 | 101879.68 | 101874.85 | -4.83 | | | 0.030 | 0.057 | 0.913 |
| | 5 | 102362.27 | 102367.15 | 4.87 | 102367.17 | 4.90 | 0.925 | 0.028 | 0.046 |
| | 5 | 102957.45 | 102955.12 | -2.33 | | | 0.039 | 0.094 | 0.867 |
| | 5 | 103957.09 | 103953.02 | -4.07 | | | 0.077 | 0.308 | 0.615 |
| | 5 | 104384.06 | 104386.87 | 2.82 | 104386.80 | 2.74 | 0.724 | 0.075 | 0.201 |
| | 5 | 104974.04 | 104972.01 | -2.03 | 104971.99 | -2.05 | 0.114 | 0.211 | 0.675 |
| | 5 | 105771.77 | 105770.13 | -1.64 | 105770.05 | -1.72 | 0.221 | 0.206 | 0.574 |
| | 5 | 106370.50 | 106374.13 | 3.64 | 106374.02 | 3.52 | 0.350 | 0.146 | 0.504 |
| | 5 | 107029.39 | 107033.00 | 3.62 | | | 0.221 | 0.149 | 0.630 |
| | 5 | 107757.82 | 107761.69 | 3.87 | | | 0.216 | 0.138 | 0.646 |
| | 5 | 108444.70 | 108450.41 | 5.71 | | | 0.258 | 0.109 | 0.633 |
| | 5 | 109110.20 | 109116.54 | 6.33 | | | 0.238 | 0.097 | 0.664 |
| | 5 | 109791.24 | 109797.45 | 6.22 | | | 0.196 | 0.088 | 0.716 |
| | 5 | 110468.36 | 110475.21 | 6.85 | | | 0.204 | 0.095 | 0.701 |
| | 5 | 111106.92 | 111114.58 | 7.67 | | | 0.248 | 0.079 | 0.673 |
| | 5 | 111645.05 | 111641.80 | -3.25 | | | 0.287 | 0.200 | 0.513 |
| *GK* | 5 | 111952.78 | 111941.70 | -11.08 | | | 0.337 | 0.143 | 0.521 |

Table 1: ($J$=6) Calculated and observed $H_2$ *singlet gerade* $e-$symmetry level energies (in $cm^{-1}$) between 90000 and 112000 $cm^{-1}$.

| state | $J$ | calculated MQDT | observed Bailly *et al.*[b] | obs-calc | observed present | obs-calc | channel character[c] s | d | p |
|---|---|---|---|---|---|---|---|---|---|
| *EF* | 6 | 99621.16 | | | | | 0.022 | 0.031 | 0.946 |
| | 6 | 100457.77 | 100461.20 | 3.43 | 100461.20 | 3.43 | 0.830 | 0.015 | 0.155 |
| | 6 | 100813.97 | 100809.50 | -4.47 | | | 0.025 | 0.039 | 0.936 |
| | 6 | 101949.82 | 101945.01 | -4.81 | | | 0.029 | 0.056 | 0.914 |
| | 6 | 102700.06 | 102701.55 | 1.49 | 102704.42 | 4.36 | 0.922 | 0.031 | 0.047 |
| | 6 | 103027.66 | 103025.52 | -2.14 | | | 0.040 | 0.081 | 0.879 |
| | 6 | 104035.99 | | | | | 0.065 | 0.206 | 0.729 |
| | 6 | 104650.20 | 104396.44[e] | -253.75[e] | 104650.43 | 0.24 | 0.647 | 0.113 | 0.240 |
| | 6 | 105078.15 | | | | | 0.152 | 0.220 | 0.628 |
| | 6 | 105891.84 | | | 105890.04 | -1.80 | 0.166 | 0.266 | 0.568 |
| | 6 | 106537.96 | | | | | 0.338 | 0.145 | 0.517 |
| | 6 | 107164.64 | | | | | 0.211 | 0.272 | 0.517 |
| | 6 | 107882.88 | | | | | 0.217 | 0.098 | 0.685 |
| | 6 | 108579.62 | | | | | 0.240 | 0.131 | 0.628 |
| | 6 | 109241.72 | | | | | 0.250 | 0.087 | 0.663 |
| | 6 | 109910.82 | | | | | 0.201 | 0.121 | 0.678 |
| | 6 | 110585.11 | | | | | 0.186 | 0.132 | 0.682 |
| | 6 | 111232.02 | | | | | 0.223 | 0.118 | 0.660 |
| | 6 | 111770.34 | | | | | 0.371 | 0.089 | 0.540 |

Table 1: ($J$=7) Calculated and observed $H_2$ *singlet gerade* $e-$symmetry level energies (in $cm^{-1}$) between 90000 and 112000 $cm^{-1}$.

| state | $J$ | calculated MQDT | observed Bailly *et al.*[b] | obs-calc | observed present | obs-calc | channel character[c] s | d | p |
|---|---|---|---|---|---|---|---|---|---|
| *EF* | 7 | 99706.04 | | | | | 0.022 | 0.036 | 0.942 |
| | 7 | 100873.97 | 100877.37 | 3.40 | 100877.37 | 3.40 | 0.898 | 0.017 | 0.085 |
| | 7 | 100897.02 | 100892.55 | -4.47 | | | 0.025 | 0.039 | 0.936 |
| | 7 | 102031.26 | 102026.57 | -4.69 | | | 0.029 | 0.068 | 0.903 |
| | 7 | 103074.84 | | | 103076.23 | 1.39 | 0.635 | 0.059 | 0.305 |
| | 7 | 103120.39 | 103106.66[e] | -13.73[e] | 103121.01[f] | 0.62 | 0.275 | 0.062 | 0.663 |
| | 7 | 104122.41 | | | | | 0.056 | 0.184 | 0.760 |
| | 7 | 104911.79 | 104989.96[e] | 78.17[e] | 104908.69 | -3.10 | 0.430 | 0.172 | 0.398 |
| | 7 | 105236.78 | | | | | 0.258 | 0.316 | 0.425 |
| | 7 | 106019.26 | | | | | 0.155 | 0.200 | 0.645 |
| | 7 | 106719.59 | | | 106721.14 | 1.55 | 0.320 | 0.091 | 0.589 |
| | 7 | 107331.25 | | | | | 0.193 | 0.411 | 0.396 |
| | 7 | 108026.24 | | | | | 0.220 | 0.087 | 0.693 |
| | 7 | 108730.00 | | | | | 0.213 | 0.176 | 0.612 |
| | 7 | 109394.79 | | | | | 0.257 | 0.070 | 0.673 |
| | 7 | 110051.16 | | | | | 0.123 | 0.488 | 0.389 |
| | 7 | 110717.02 | | | | | 0.192 | 0.081 | 0.727 |
| | 7 | 111370.49 | | | | | 0.147 | 0.351 | 0.503 |
| | 7 | 111928.70 | | | | | 0.411 | 0.065 | 0.524 |

Table 1: ($J$=8) Calculated and observed $H_2$ *singlet gerade* $e-$symmetry level energies (in $cm^{-1}$) between 90000 and 112000 $cm^{-1}$.

| state | $J$ | calculated MQDT | observed Bailly *et al.*[b] | obs-calc | observed present | obs-calc | channel character[c] s | d | p |
|---|---|---|---|---|---|---|---|---|---|
| $EF$ | 8 | 99802.69 | | | | | 0.022 | 0.030 | 0.948 |
| | 8 | 100991.72 | | | | | 0.024 | 0.040 | 0.936 |
| | 8 | 101340.42 | 101343.82 | 3.41 | 101343.82 | 3.40 | 0.914 | 0.018 | 0.069 |
| | 8 | 102123.98 | | | | | 0.028 | 0.053 | 0.918 |
| | 8 | 103197.49 | 103199.24 | 1.75 | | | 0.039 | 0.086 | 0.875 |
| | 8 | 103521.12 | | | 103525.37 | 4.25 | 0.912 | 0.035 | 0.053 |
| | 8 | 104218.38 | 103838.57[e] | -379.81[e] | | | 0.038 | 0.390 | 0.572 |
| | 8 | 105107.35 | | | | | 0.194 | 0.222 | 0.584 |
| | 8 | 105498.98 | | | | | 0.570 | 0.067 | 0.363 |
| | 8 | 106160.16 | | | | | 0.148 | 0.227 | 0.625 |
| | 8 | 106903.80 | | | | | 0.259 | 0.096 | 0.646 |
| | 8 | 107529.44 | | | 107537.79 | 8.35 | 0.255 | 0.272 | 0.472 |
| | 8 | 108191.76 | | | | | 0.235 | 0.084 | 0.681 |
| | 8 | 108893.72 | | | | | 0.165 | 0.313 | 0.522 |
| | 8 | 109566.23 | | | | | 0.248 | 0.076 | 0.676 |
| | 8 | 110213.71 | | | | | 0.223 | 0.127 | 0.651 |
| | 8 | 110865.49 | | | | | 0.198 | 0.075 | 0.728 |
| | 8 | 111518.38 | | | | | 0.180 | 0.105 | 0.715 |

Table 1: ($J$=9) Calculated and observed $H_2$ *singlet gerade* $e-$symmetry level energies (in $cm^{-1}$) between 90000 and 112000 $cm^{-1}$.

| state | $J$ | calculated MQDT | observed Bailly *et al.*[b] | obs-calc | observed present | obs-calc | channel character[d] s | d | p |
|---|---|---|---|---|---|---|---|---|---|
| $EF$ | 9 | 99911.06 | | | | | 0.021 | 0.030 | 0.949 |
| | 9 | 101097.75 | | | | | 0.024 | 0.037 | 0.939 |
| | 9 | 101853.76 | 101857.17 | 3.42 | 101857.17 | 3.41 | 0.904 | 0.019 | 0.077 |
| | 9 | 102227.83 | | | | | 0.028 | 0.050 | 0.922 |
| | 9 | 103300.78 | | | | | 0.035 | 0.082 | 0.882 |
| | 9 | 103990.98 | | | 103994.68 | 3.70 | 0.889 | 0.045 | 0.065 |
| | 9 | 104326.46 | | | 104323.32 | -3.14 | 0.052 | 0.229 | 0.719 |
| | 9 | 105251.99 | | | | | 0.063 | 0.549 | 0.389 |
| | 9 | 105825.68 | | | 105826.53 | 0.85 | 0.553 | 0.086 | 0.361 |
| | 9 | 106331.35 | | | | | 0.162 | 0.360 | 0.478 |
| | 9 | 107086.08 | | | | | 0.206 | 0.121 | 0.672 |
| | 9 | 107749.45 | | | | | 0.247 | 0.270 | 0.483 |
| | 9 | 108384.97 | | | 108386.73 | 1.76 | 0.259 | 0.090 | 0.651 |
| | 9 | 109071.47 | | | | | 0.204 | 0.127 | 0.669 |
| | 9 | 109751.08 | | | | | 0.227 | 0.093 | 0.680 |
| | 9 | 110397.71 | | | | | 0.237 | 0.091 | 0.672 |
| | 9 | 111033.44 | | | | | 0.208 | 0.090 | 0.703 |
| | 9 | 111675.42 | | | | | 0.175 | 0.085 | 0.739 |

Table 1: ($J$=10) Calculated and observed $H_2$ *singlet gerade e*−symmetry level energies (in $cm^{-1}$) between 90000 and 112000 $cm^{-1}$.

| state | $J$ | calculated MQDT | observed Bailly *et al.*[b] | obs-calc | observed present | obs-calc | channel character[d] s | d | p |
|---|---|---|---|---|---|---|---|---|---|
| $EF$ | 10 | 100031.02 | | | | | 0.021 | 0.029 | 0.950 |
| | 10 | 101215.08 | | | | | 0.023 | 0.036 | 0.940 |
| | 10 | 102342.55 | | | | | 0.028 | 0.048 | 0.923 |
| | 10 | 102410.61 | 102414.05 | 3.44 | 102414.05 | 3.44 | 0.839 | 0.019 | 0.143 |
| | 10 | 103414.26 | | | 103420.55[f] | 6.29 | 0.034 | 0.074 | 0.892 |
| | 10 | 104411.37 | | | | | 0.188 | 0.135 | 0.677 |
| | 10 | 104530.58 | | | 104534.09 | 3.51 | 0.727 | 0.043 | 0.229 |
| | 10 | 105386.11 | | | | | 0.079 | 0.214 | 0.707 |
| | 10 | 106128.28 | | | | | 0.355 | 0.146 | 0.499 |
| | 10 | 106570.70 | | | | | 0.226 | 0.457 | 0.317 |
| | 10 | 107272.72 | | | | | 0.182 | 0.150 | 0.668 |
| | 10 | 107975.18 | | | | | 0.254 | 0.132 | 0.614 |
| | 10 | 108608.19 | | | | | 0.270 | 0.118 | 0.612 |
| | 10 | 109267.46 | | | | | 0.221 | 0.096 | 0.683 |
| | 10 | 109945.65 | | | | | 0.196 | 0.153 | 0.651 |
| | 10 | 110598.46 | | | | | 0.230 | 0.081 | 0.689 |
| | 10 | 111223.69 | | | | | 0.184 | 0.250 | 0.565 |
| | 10 | 111846.26 | | | | | 0.185 | 0.087 | 0.729 |

Table 1: ($J$=11) Calculated and observed $H_2$ *singlet gerade* $e-$symmetry level energies (in $cm^{-1}$) between 90000 and 112000 $cm^{-1}$.

| state | $J$ | calculated MQDT | observed Bailly *et al.*[b] | obs-calc | observed present | obs-calc | channel character[d] s | d | p |
|---|---|---|---|---|---|---|---|---|---|
| $EF$ | 11 | 100162.41 | | | | | 0.021 | 0.029 | 0.951 |
| | 11 | 101343.52 | | | | | 0.023 | 0.036 | 0.942 |
| | 11 | 102468.22 | | | | | 0.027 | 0.048 | 0.926 |
| | 11 | 103007.02 | 103010.50 | 3.48 | 103010.50 | 3.48 | 0.888 | 0.021 | 0.091 |
| | 11 | 103538.14 | | | | | 0.032 | 0.089 | 0.879 |
| | 11 | 104553.66 | | | | | 0.049 | 0.140 | 0.811 |
| | 11 | 105049.91 | | | 105052.90 | 3.00 | 0.847 | 0.057 | 0.096 |
| | 11 | 105526.99 | | | 105523.80 | -3.19 | 0.058 | 0.413 | 0.529 |
| | 11 | 106357.19 | | | | | 0.180 | 0.216 | 0.604 |
| | 11 | 106892.16 | | | 106894.85 | 2.69 | 0.439 | 0.134 | 0.427 |
| | 11 | 107481.65 | | | | | 0.205 | 0.168 | 0.628 |
| | 11 | 108197.20 | | | | | 0.220 | 0.104 | 0.675 |
| | 11 | 108853.01 | | | | | 0.227 | 0.244 | 0.528 |
| | 11 | 109488.31 | | | | | 0.246 | 0.084 | 0.670 |
| | 11 | 110151.35 | | | | | 0.173 | 0.230 | 0.597 |
| | 11 | 110808.92 | | | | | 0.210 | 0.092 | 0.698 |
| | 11 | 111434.77 | | | | | 0.204 | 0.186 | 0.610 |

Table 1: ($J$=12) Calculated and observed $H_2$ *singlet gerade e*−symmetry level energies (in $cm^{-1}$) between 90000 and 112000 $cm^{-1}$.

| state | $J$ | calculated MQDT | observed Bailly *et al.*[b] | obs-calc | observed present | obs-calc | channel character[d] s | d | p |
|---|---|---|---|---|---|---|---|---|---|
| $EF$ | 12 | 100305.16 | | | | | 0.020 | 0.029 | 0.951 |
| | 12 | 101483.13 | | | | | 0.022 | 0.035 | 0.942 |
| | 12 | 102604.59 | | | | | 0.026 | 0.046 | 0.928 |
| | 12 | 103638.31 | 103641.54 | 3.23 | 103641.54 | 3.23 | 0.869 | 0.026 | 0.105 |
| | 12 | 103673.39 | | | 103672.48[f] | -0.91 | 0.056 | 0.067 | 0.877 |
| | 12 | 104689.69 | | | | | 0.042 | 0.117 | 0.841 |
| | 12 | 105553.91 | | | 105551.50 | -2.41 | 0.425 | 0.194 | 0.381 |
| | 12 | 105730.20 | | | 105732.04 | 1.84 | 0.278 | 0.343 | 0.379 |
| | 12 | 106543.90 | | | | | 0.109 | 0.272 | 0.619 |
| | 12 | 107220.95 | | | | | 0.364 | 0.100 | 0.536 |
| | 12 | 107743.64 | | | | | 0.160 | 0.548 | 0.292 |
| | 12 | 108421.33 | | | | | 0.206 | 0.101 | 0.692 |
| | 12 | 109102.88 | | | | | 0.218 | 0.189 | 0.593 |
| | 12 | 109735.58 | | | | | 0.262 | 0.087 | 0.651 |
| | 12 | 110374.14 | | | | | 0.145 | 0.389 | 0.466 |
| | 12 | 111025.62 | | | | | 0.195 | 0.090 | 0.714 |
| | 12 | 111658.36 | | | | | 0.200 | 0.144 | 0.656 |

Table 1: ($J$=13) Calculated and observed $H_2$ *singlet gerade e*−symmetry level energies (in $cm^{-1}$) between 90000 and 112000 $cm^{-1}$.

| state | $J$ | calculated MQDT | observed Bailly *et al.*[b] | obs-calc | observed present | obs-calc | channel s | character[d] d | p |
|---|---|---|---|---|---|---|---|---|---|
| *EF* | 13 | 100458.95 | | | | | 0.020 | 0.027 | 0.953 |
| | 13 | 101633.31 | | | | | 0.022 | 0.034 | 0.945 |
| | 13 | 102751.27 | | | | | 0.025 | 0.044 | 0.931 |
| | 13 | 103816.31 | | | | | 0.031 | 0.063 | 0.906 |
| | 13 | 104303.85 | 104303.02 | -0.83 | 104307.45 | 3.60 | 0.718 | 0.021 | 0.261 |
| | 13 | 104833.88 | | | | | 0.038 | 0.129 | 0.833 |
| | 13 | 105777.60 | | | | | 0.078 | 0.191 | 0.731 |
| | 13 | 106230.84 | | | 106232.97 | 2.13 | 0.733 | 0.067 | 0.199 |
| | 13 | 106729.75 | | | 106727.84 | -1.91 | 0.094 | 0.369 | 0.536 |
| | 13 | 107492.66 | | | | | 0.218 | 0.140 | 0.642 |
| | 13 | 108067.27 | | | | | 0.358 | 0.138 | 0.504 |
| | 13 | 108667.61 | | | | | 0.232 | 0.127 | 0.640 |
| | 13 | 109349.33 | | | | | 0.217 | 0.081 | 0.702 |
| | 13 | 109998.65 | | | | | 0.237 | 0.137 | 0.626 |
| | 13 | 110620.52 | | | | | 0.228 | 0.118 | 0.654 |
| | 13 | 111252.61 | | | | | 0.160 | 0.263 | 0.577 |
| | 13 | 111885.52 | | | | | 0.189 | 0.097 | 0.714 |

Table 1: ($J$=14) Calculated and observed $H_2$ *singlet gerade* $e-$symmetry level energies (in $cm^{-1}$) between 90000 and 112000 $cm^{-1}$.

| state | $J$ | calculated MQDT | observed Bailly *et al.*[b] | obs-calc | observed present | obs-calc | channel character[d] s | d | p |
|---|---|---|---|---|---|---|---|---|---|
| $EF$ | 14 | 100623.71 | | | | | 0.019 | 0.026 | 0.954 |
| | 14 | 101794.16 | | | | | 0.021 | 0.033 | 0.946 |
| | 14 | 102908.23 | | | | | 0.025 | 0.042 | 0.933 |
| | 14 | 103970.46 | | | | | 0.030 | 0.058 | 0.912 |
| | 14 | 104975.31 | | | 104973.02 | -2.29 | 0.277 | 0.163 | 0.560 |
| | 14 | 105007.52 | | | 105009.27 | 1.75 | 0.571 | 0.056 | 0.374 |
| | 14 | 105940.18 | | | | | 0.051 | 0.210 | 0.739 |
| | 14 | 106722.95 | | | 106719.61 | -3.34 | 0.324 | 0.291 | 0.386 |
| | 14 | 107001.52 | | | 107004.11 | 2.59 | 0.410 | 0.123 | 0.467 |
| | 14 | 107722.39 | | | | | 0.154 | 0.148 | 0.698 |
| | 14 | 108393.59 | | | | | 0.294 | 0.128 | 0.578 |
| | 14 | 108960.81 | | | | | 0.259 | 0.236 | 0.505 |
| | 14 | 109601.56 | | | | | 0.208 | 0.121 | 0.671 |
| | 14 | 110262.22 | | | | | 0.187 | 0.228 | 0.584 |
| | 14 | 110887.62 | | | | | 0.238 | 0.091 | 0.671 |
| | 14 | 111498.44 | | | | | 0.209 | 0.113 | 0.677 |

Table 1: ($J$=15) Calculated and observed $H_2$ *singlet gerade* $e-$symmetry level energies (in $cm^{-1}$) between 90000 and 112000 $cm^{-1}$.

| state | $J$ | calculated MQDT | observed Bailly *et al.*[b] | obs-calc | observed present | obs-calc | channel character[d] s | d | p |
|---|---|---|---|---|---|---|---|---|---|
| $EF$ | 15 | 100799.23 | | | | | 0.019 | 0.026 | 0.956 |
| | 15 | 101965.41 | | | | | 0.021 | 0.032 | 0.948 |
| | 15 | 103075.33 | | | | | 0.024 | 0.045 | 0.932 |
| | 15 | 104134.28 | | | | | 0.029 | 0.054 | 0.917 |
| | 15 | 105147.84 | | | | | 0.035 | 0.093 | 0.872 |
| | 15 | 105711.53 | | | 105715.15 | 3.62 | 0.879 | 0.034 | 0.087 |
| | 15 | 106106.03 | | | | | 0.048 | 0.174 | 0.778 |
| | 15 | 106981.22 | | | | | 0.101 | 0.251 | 0.648 |
| | 15 | 107492.96 | | | 107494.19 | 1.23 | 0.610 | 0.075 | 0.315 |
| | 15 | 107961.59 | | | 107962.14 | 0.56 | 0.138 | 0.392 | 0.471 |
| | 15 | 108676.41 | | | | | 0.205 | 0.125 | 0.669 |
| | 15 | 109290.47 | | | 109293.90 | 3.43 | 0.293 | 0.153 | 0.555 |
| | 15 | 109880.99 | | | | | 0.251 | 0.104 | 0.645 |
| | 15 | 110524.77 | | | | | 0.200 | 0.119 | 0.681 |
| | 15 | 111160.88 | | | | | 0.215 | 0.107 | 0.678 |
| | 15 | 111766.06 | | | | | 0.223 | 0.109 | 0.668 |

Table 1: ($J$=16) Calculated and observed $H_2$ *singlet gerade e*−symmetry level energies (in $cm^{-1}$) between 90000 and 112000 $cm^{-1}$.

| state | $J$ | calculated MQDT | observed Bailly *et al.*[b] | obs-calc | observed present | obs-calc | channel character[d] s | d | p |
|---|---|---|---|---|---|---|---|---|---|
| $EF$ | 16 | 100985.51 | | | | | 0.018 | 0.025 | 0.956 |
| | 16 | 102147.13 | | | | | 0.020 | 0.031 | 0.949 |
| | 16 | 103252.19 | | | | | 0.023 | 0.039 | 0.938 |
| | 16 | 104307.64 | | | | | 0.027 | 0.063 | 0.910 |
| | 16 | 105318.94 | | | | | 0.033 | 0.081 | 0.886 |
| | 16 | 106269.01 | | | | | 0.065 | 0.154 | 0.781 |
| | 16 | 106453.47 | | | 106457.32 | 3.85 | 0.664 | 0.026 | 0.310 |
| | 16 | 107173.34 | | | | | 0.059 | 0.311 | 0.631 |
| | 16 | 107920.96 | | | 107917.60 | -3.36 | 0.277 | 0.168 | 0.555 |
| | 16 | 108317.85 | | | | | 0.443 | 0.112 | 0.445 |
| | 16 | 108937.20 | | | 108937.93 | 0.73 | 0.170 | 0.182 | 0.648 |
| | 16 | 109605.97 | | | 109607.40 | 1.43 | 0.240 | 0.111 | 0.649 |
| | 16 | 110198.13 | | | 110202.77 | 4.64 | 0.259 | 0.180 | 0.562 |
| | 16 | 110801.50 | | | 110806.31 | 4.81 | 0.207 | 0.166 | 0.628 |
| | 16 | 111431.36 | | | | | 0.141 | 0.357 | 0.501 |

Table 1: ($J$=17) Calculated and observed $H_2$ *singlet gerade* $e-$symmetry level energies (in $cm^{-1}$) between 90000 and 112000 $cm^{-1}$.

| state | $J$ | calculated MQDT | observed Bailly *et al.*[b] | obs-calc | observed present | obs-calc | channel character[d] s | d | p |
|---|---|---|---|---|---|---|---|---|---|
| $EF$ | 17 | 101181.92 | | | | | 0.018 | 0.024 | 0.958 |
| | 17 | 102338.46 | | | | | 0.019 | 0.030 | 0.950 |
| | 17 | 103438.70 | | | | | 0.023 | 0.037 | 0.940 |
| | 17 | 104490.25 | | | | | 0.027 | 0.049 | 0.924 |
| | 17 | 105498.26 | | | | | 0.031 | 0.069 | 0.899 |
| | 17 | 106451.42 | | | | | 0.038 | 0.156 | 0.806 |
| | 17 | 107184.14 | | | 107186.40 | 2.26 | 0.725 | 0.060 | 0.214 |
| | 17 | 107372.62 | | | | | 0.115 | 0.170 | 0.715 |
| | 17 | 108182.17 | | | | | 0.106 | 0.274 | 0.621 |
| | 17 | 108779.91 | | | 108780.07 | 0.16 | 0.411 | 0.085 | 0.503 |
| | 17 | 109240.39 | | | | | 0.188 | 0.423 | 0.388 |
| | 17 | 109892.32 | | | | | 0.182 | 0.141 | 0.678 |
| | 17 | 110523.51 | | | 110526.86 | 3.35 | 0.234 | 0.159 | 0.607 |
| | 17 | 111108.18 | | | | | 0.245 | 0.133 | 0.622 |
| | 17 | 111708.48 | | | | | 0.205 | 0.100 | 0.696 |

Table 1: ($J$=18) Calculated and observed $H_2$ *singlet gerade* $e-$symmetry level energies (in $cm^{-1}$) between 90000 and 112000 $cm^{-1}$.

| state | $J$ | calculated MQDT | observed Bailly *et al.*[b] | obs-calc | observed present | obs-calc | channel character[d] s | d | p |
|---|---|---|---|---|---|---|---|---|---|
| $EF$ | 18 | 101388.55 | | | | | 0.017 | 0.023 | 0.960 |
| | 18 | 102540.58 | | | | | 0.019 | 0.031 | 0.950 |
| | 18 | 103634.63 | | | | | 0.022 | 0.036 | 0.942 |
| | 18 | 104681.91 | | | | | 0.026 | 0.045 | 0.929 |
| | 18 | 105685.94 | | | | | 0.030 | 0.072 | 0.898 |
| | 18 | 106637.73 | | | | | 0.034 | 0.146 | 0.820 |
| | 18 | 107534.15 | | | | | 0.060 | 0.182 | 0.759 |
| | 18 | 107960.10 | | | | | 0.816 | 0.050 | 0.134 |
| | 18 | 108402.85 | | | | | 0.072 | 0.380 | 0.548 |
| | 18 | 109132.89 | | | | | 0.204 | 0.136 | 0.659 |
| | 18 | 109649.64 | | | | | 0.399 | 0.109 | 0.492 |
| | 18 | 110188.50 | | | | | 0.147 | 0.420 | 0.433 |
| | 18 | 110827.08 | | | | | 0.203 | 0.103 | 0.694 |
| | 18 | 111431.80 | | | | | 0.219 | 0.189 | 0.592 |

Table 1: ($J$=19) Calculated and observed $H_2$ *singlet gerade* $e-$symmetry level energies (in $cm^{-1}$) between 90000 and 112000 $cm^{-1}$.

| state | $J$ | calculated MQDT | observed Bailly *et al.*[b] | obs-calc | observed present | obs-calc | channel s | character[d] d | p |
|---|---|---|---|---|---|---|---|---|---|
| $EF$ | 19 | 101604.93 | | | | | 0.016 | 0.022 | 0.961 |
| | 19 | 102750.68 | | | | | 0.018 | 0.028 | 0.954 |
| | 19 | 103839.92 | | | | | 0.021 | 0.050 | 0.929 |
| | 19 | 104882.40 | | | | | 0.025 | 0.043 | 0.933 |
| | 19 | 105882.38 | | | | | 0.023 | 0.250 | 0.727 |
| | 19 | 106831.19 | | | | | 0.034 | 0.086 | 0.880 |
| | 19 | 107731.52 | | | | | 0.039 | 0.246 | 0.715 |
| | 19 | 108543.04 | | | | | 0.194 | 0.169 | 0.637 |
| | 19 | 108773.91 | | | 108777.75 | 3.84 | 0.622 | 0.059 | 0.319 |
| | 19 | 109394.27 | | | | | 0.112 | 0.244 | 0.645 |
| | 19 | 110045.68 | | | | | 0.276 | 0.102 | 0.623 |
| | 19 | 110553.08 | | | | | 0.171 | 0.536 | 0.294 |
| | 19 | 111126.83 | | | | | 0.209 | 0.107 | 0.684 |
| | 19 | 111742.65 | | | | | 0.195 | 0.139 | 0.666 |
